# Supplementary material for: Customizing the angular memory effect for scattering media
Source: arXiv:2010.08290 ancillary file (2021-05-27)
Supplement: Supplementary file 1 [file 2021_supplementary_Customizing_angular_memory_effect_for_scattering_media.pdf]

# Customizing the angular memory effect for scattering media: supplementary material


Hasan Yılmaz,[1,2] Matthias Kühmayer,[3] Chia Wei Hsu,[4] Stefan Rotter,[3] and Hui Cao[1,*]

[1] *Department of Applied Physics, Yale University, New Haven, Connecticut 06520, USA*
[2] *Institute of Materials Science and Nanotechnology, National Nanotechnology Research Center (UNAM), Bilkent University, 06800 Ankara, Turkey*
[3] *Institute for Theoretical Physics, Vienna University of Technology (TU Wien), A-1040 Vienna, Austria*
[4] *Ming Hsieh Department of Electrical and Computer Engineering, University of Southern California, Los Angeles, California 90089, USA*



(Dated: May 27, 2021)


This document provides supplementary information to 'Customizing the angular memory effect for scattering media'. Here, we elaborate on the experimental setup, the measurement procedure, data analysis, and the experimental results.

## A. Scattering sample

The scattering sample is made of densely-packed zinc oxide (ZnO) nanoparticles (average diameter $\simeq$ 200 nm), deposited on a cover slip (thickness 170 µm). The ZnO layer thickness is about 10 µm. The average transmittance at $\lambda = 532$ nm is approximately 0.2.

## B. Experimental setup

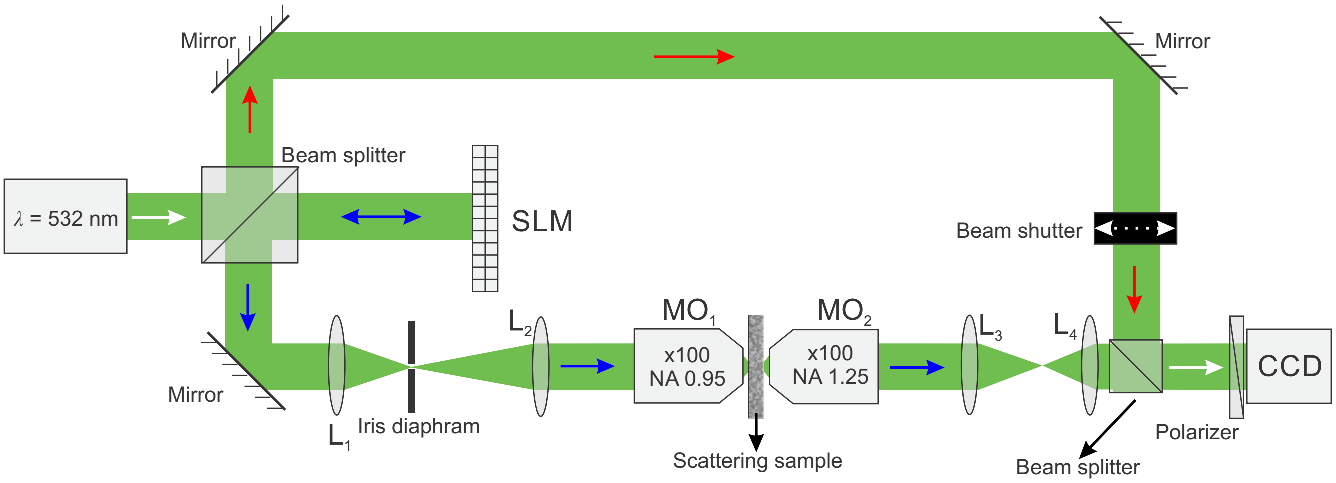


FIG. S1. **A sketch of our interferometric setup.** A reflective phase-only spatial light modulator (SLM) modulates the phase front of a monochromatic laser beam ($\lambda = 532$ nm). The field transmission matrix of the scattering sample is measured in $k$ space with the SLM and the CCD camera. $MO_{1,2}$: microscope objectives. $L_{1-4}$: lenses.

A sketch of our experimental setup is presented in Fig. S1. A linearly-polarized monochromatic laser beam (Coherent, Compass 215M-50 SL) with wavelength $\lambda = 532$ nm is expanded and collimated before splitting into two arms of the interferometer. The beam launched to the sample arm illuminates a SLM (Hamamatsu, X10468-01). The reflected beam is directed to the sample. The SLM plane is imaged onto the pupil of a microscope objective $MO_1$ (Nikon CF Plan 100×, numerical aperture $NA_{in} = 0.95$) by a pair of lenses $L_1$ and $L_2$ (with focal lengths $f_1 = 100$ mm and $f_2 = 250$ mm). An iris diaphragm between $L_1$ and $L_2$ blocks high-order diffractions from the SLM.


* hui.cao@yale.edu

The light transmitted through the sample is collected by an oil-immersion microscope objective $MO_2$ (Edmund Optics DIN Achromatic 100×, $NA_{out} = 1.25$) and collimated by a pair of lens $L_5$ ($f_5 = 200$ mm) and $L_6$ ($f_6 = 150$ mm). It then recombines with the reference beam from the other arm of the interferometer. Their interference pattern is recorded by a CCD camera (Allied Vision, Manta G-031B), which is placed at the Fourier plane of the back (output) surface of the sample. A linear polarizer in front of the camera selects one polarization component of the light.

### C. Transmission matrix measurement

The field transmission matrix from the SLM to the CCD camera is measured in Hadamard basis, with a four-phase-shift interferometry method. 2415 SLM macropixels within a circle are imaged onto the entrance pupil of $MO_1$, covering the entire pupil. Among them, we use $32 \times 32 = 1024$ macropixels inside a central square as input channels. Each macropixel consists of $9 \times 9$ SLM pixels. A high-spatial-frequency phase grating is written outside the central square on the SLM to diffract the light away from the iris diaphram.

By applying four global phases in between 0 and $2\pi$ to the Hadamard phase patterns on the $32\times32$ SLM macropixels, we retrieve the phase difference between the transmitted field pattern and the reference beam with a flat phase front from their interference patterns on the CCD camera. Finally, we block the reference beam with a beam shutter, and measure the transmitted intensity patterns of the 1024 Hadamard phase pattern inputs. Combining the measured phase pattern and the amplitude pattern of the transmitted light, we obtain the complex field pattern.

In this setup, we modulate a single linear polarization of light at the input, and detect a single linear polarization of light at the output. Experimentally we measure the transmitted field pattern within a square on the CCD camera that has $64 \times 64 = 4096$ pixels. The transmission matrix $t$ is a $N_o \times N_i$ matrix, where $N_i = 1024$ is the number of SLM macropixels, $N_o = 4096$ is the number of CCD camera pixels.

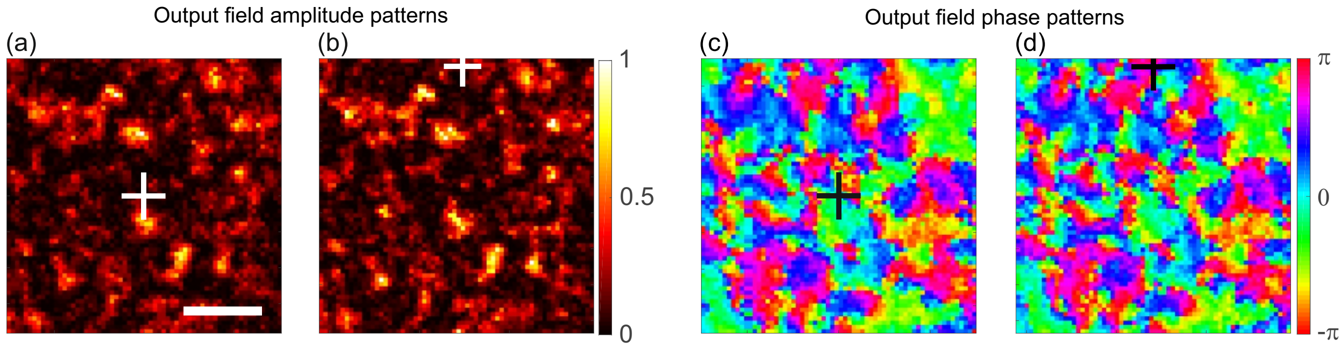


FIG. S2. **Output patterns of an angular memory eigenstate.** Amplitude **(a,b)** and phase **(c,d)** patterns of the transmitted complex fields in Fig. 2(b,c) of the main text are shown separately. The Pearson correlation coefficient between the amplitude patterns is 0.82 and between the phase patterns is 0.83. The horizontal and vertical axes represent $k_{o,x}$ and $k_{o,y}$, the components of the output wavevector in $x$ and $y$ directions, respectively. The white/black plus signs mark the origin: $k_{o,x} = 0$, $k_{o,y} = 0$. The scale bar represents $k = 0.05(2\pi/\lambda)$.

### D. Rotation operator and edge effects

Here we elaborate on the rotation operators $X$ that tilt the incoming and outgoing field profiles, in Eqs. (1) and (2) of the main text. $X$ can be expressed as a matrix. For the illustration purpose, let us first consider a 2D scattering medium whose 1D cross-section is parallel to $y$ axis and light transmitting along $z$ axis. The transmission matrix $t$ is given in the momentum space, mapping the input transverse wavevectors $k_y$ to the output ones. Tilting the incident wavefront by an angle $\theta_i$ corresponds to shifting input $k_y$ to $k_y + \Delta k_y$, where $\Delta k_y = k \sin\theta_i$ and $k = 2\pi/\lambda$. Since each column of the transmission matrix represents an input $k_y$, a shift of input $k_y$ is equivalent to a lateral shift of matrix columns, which is done by multiplying the $t$ matrix by a matrix $X$ whose elements are equal to zero except on a line parallel to the matrix diagonal. Its distance to the diagonal is determined by the amount of shift $\Delta = k \sin\theta_i/\delta k_y$, where $\delta k_y$ is the sampling step of input $k_y$ for the $t$ matrix. The matrix $X$ element $X_{p\,q} = \delta_{p\,q+\Delta}$, i.e., only for $p = q + \Delta$, the value is equal to 1, otherwise it is equal to 0. Similar argument holds for tilting the transmitted wavefront by shifting the $t$ matrix rows. Next we consider a 3D scattering medium whose 2D cross-section is parallel to $x - y$ plane. Although the expression of matrix $X$ is more complicated, its function is to move the transmission

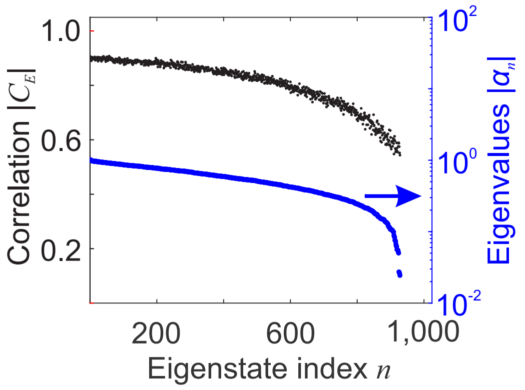


FIG. S3. **Correlations and eigenvalues of the angular memory eigenstates.** The angular memory operator $Q$, which is identical to that in Fig. 2 of the main text, has 1024 eigenstates, are ordered by their eigenvalue amplitude $|\alpha_n|$ (blue). Their angular correlation coefficient $|C_E|$ (black) drops with $|\alpha_n|$. The first eigenstate ($n = 1$) with the highest $|\alpha_n|$ exhibit the strongest angular correlation.

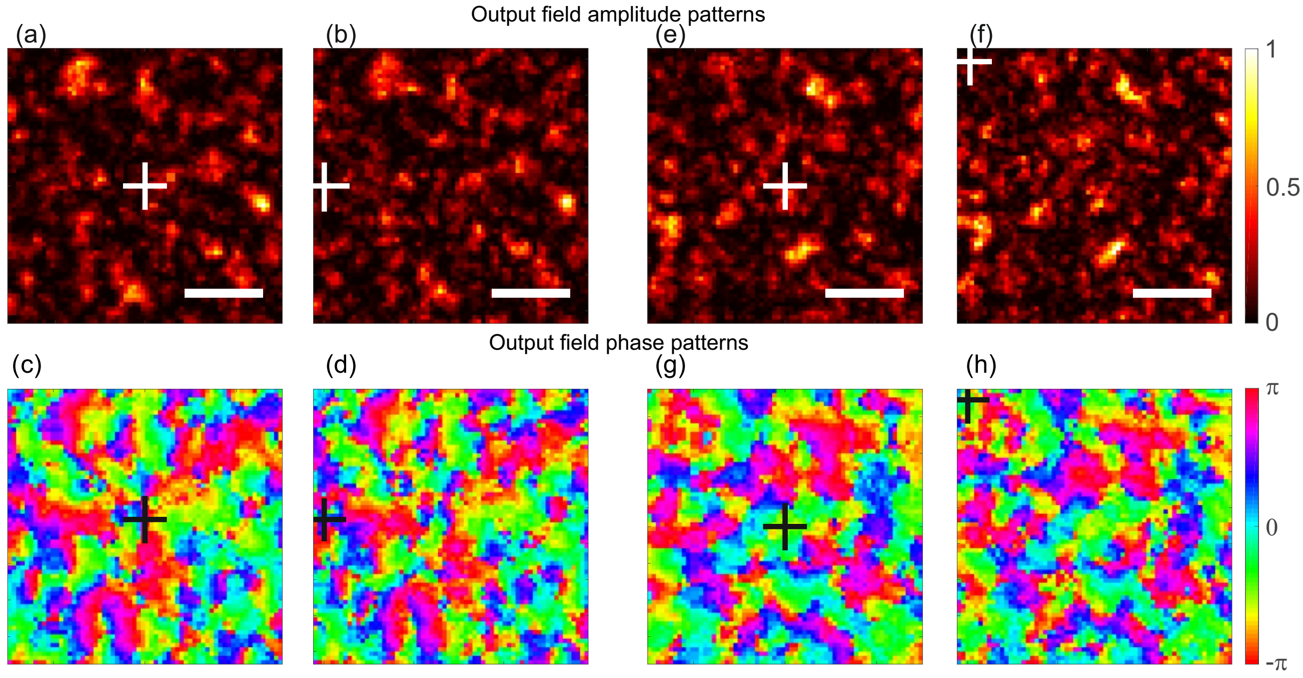


FIG. S4. **Two angular memory eigenstates with different tilt directions of the input and the output wavefronts. (a-d)** Amplitude (a,b) and phase (c,d) patterns of the transmitted fields for an angular memory eigenstate with the input field tilted in $-y$ by 7.8° and the output field tilted in $x$ by 7.1° are shown. **(e-h)** Amplitude (e,f) and phase (g,h) patterns of the transmitted fields for an angular memory eigenstate with the input field tilted in $-y$ by 7.8° and the output field tilted in the diagonal direction $\hat{x} + \hat{y}$ by 7.1° are shown. The white/black plus signs mark the origin, and the scale bars are identical to those in Fig. S2.

matrix elements $t_{m\,n}$ to $t_{m\,n+\Delta}$ for tilting the input wavefront, or to $t_{m+\Delta\,n}$ for tilting the output wavefront, where $\Delta$ is proportional to the tilt angle.

To avoid any edge effect in tilting, we experimentally measure the transmission matrix over a large angular range, e.g., from $-20°$ to $20°$ for both input and output angles, and then crop the matrix to $-10°$ to $10°$. While shifting the matrix columns or rows, we resort to the original large matrix and shift the columns or rows first before cropping. This will allow us to tilt from $-10°$ to $10°$ without any edge effect.

### E. Angular memory operator

In the main text, we show that the additional term $(t^\dagger t)^{-1}$ counter-balances the increase of the denominator of the angular correlation coefficient. Alternatively, one can use $\{[X^\dagger(\tilde{\theta}_o)tX(\tilde{\theta}_i)]^\dagger X^\dagger(\tilde{\theta}_o)tX(\tilde{\theta}_i)\}^{-1}$, and obtain the same operator given in Eq. 2 of the main text. First, we start with the definition $Q'$ below by multiplying $Q_0$ with $\{[X^\dagger(\tilde{\theta}_o)tX(\tilde{\theta}_i)]^\dagger X^\dagger(\tilde{\theta}_o)tX(\tilde{\theta}_i)\}^{-1}$ from the right as

$$Q' \equiv t^\dagger X^\dagger(\tilde{\theta}_o)tX(\tilde{\theta}_i)\{[X^\dagger(\tilde{\theta}_o)tX(\tilde{\theta}_i)]^\dagger X^\dagger(\tilde{\theta}_o)tX(\tilde{\theta}_i)\}^{-1}. \quad \text{(S1)}$$

When $t$ is an $N_o \times N_i$ square matrix ($N_o = N_i$), $[t^\dagger]^{-1}$ exists, therefore the relation above can be simplified to

$$Q' = t^\dagger X^\dagger(\tilde{\theta}_o)[t^\dagger]^{-1}X(\tilde{\theta}_i). \quad \text{(S2)}$$

Using the left eigenvalue decomposition as $\langle V_n| t^\dagger X^\dagger(\tilde{\theta}_o)[t^\dagger]^{-1}X(\tilde{\theta}_i) = \langle V_n| \alpha'_n$ we obtain $\langle V_n| t^\dagger = \langle V_n| [X^\dagger(\tilde{\theta}_i)t^\dagger X(\tilde{\theta}_o)]\alpha'_n$, which is identical to

$$t|V_n\rangle = \alpha'^\dagger_n[X^\dagger(\tilde{\theta}_o)tX(\tilde{\theta}_i)]|V_n\rangle. \quad \text{(S3)}$$

### F. Angular memory eigenstates

Fig. 2 in the main text shows that when the incident wavefront of an angular memory eigenstate is tilted by 7.8° in $-y$ direction, the transmitted field pattern tilts by 7.1° in $+y$ direction. In Fig. 2(b,c), the complex fields in transmission are plotted in such a way that the brightness is proportional to the field amplitude and the color represents phase. In Fig. S2(a-d), we plot the amplitude and phase patterns of the transmitted fields to show their similarities separately.

Here, the measured transmission matrix $t$ is a rectangular matrix with $N_o = 4096 > N_i = 1024$. When $t$ is a rectangular matrix with $N_o > N_i$, we construct the angular memory operator $Q(\tilde{\theta}_i, \tilde{\theta}_o) = (t^\dagger t)^{-1}t^\dagger X^\dagger(\tilde{\theta}_o)tX(\tilde{\theta}_i)$ using the left inverse of $t_{4096\times1024}$ as $(t^\dagger t)^{-1}t^\dagger$. $Q$ has 1024 eigenvalues $\alpha_n$ ($n = 1, 2, ..., 1024$), and the corresponding eigenstates are ordered by $|\alpha_n|$ from high to low, as shown in Fig. S3. The angular correlation $|C_E|$ increases with $|\alpha_n|$, and the first eigenstate ($n = 1$) with the largest $|\alpha_1|$ has the strongest correlation, as shown in Fig. 2 of the main text.

### G. Customized angular memory effect

In Fig. S2, input and output wavefronts are tilted in opposite directions along the $y$ axis. In Fig. S4(a-h), we construct different eigenstates of $Q$ to customize the angular memory effect, such that when the input wavefront is tilted in $y$ direction, the output wavefront tilts in $x$ direction or diagonal direction $\hat{x} + \hat{y}$.

### H. Phase-only modulation with truncated matrix inversion

The left inverse $(t^\dagger t)^{-1}t^\dagger$ reduces to $t^{-1}$, when $t$ is a square matrix with $N_o = N_i$ such as in Fig. 3 of the main text. Perfect angular correlation $|C_E| = 1$ is achieved with full-field (amplitude and phase) modulation of the input wavefront in Fig. 3(a). However, phase-only modulation of the input field reduces $|C_E|$ significantly, as seen in Fig. 3(b). This is caused by the low-transmission eigenchannels constituting an eigenvector of angular memory operator $Q$.

In order to couple light into angular memory eigenstates with phase-only modulation of the incident wavefront in experiments, we must discard the low-transmission eigenchannels that are sensitive to the absence of amplitude modulation. To remove the low-transmission eigenchannels, we first conduct the singular value decomposition $t = U_n\Sigma_n V_n^\dagger$, where the columns of $V_n$ and $U_n$ represent the input and the output wavefronts of the transmission eigenchannels, respectively, and the diagonal elements of $\Sigma_n$ gives the singular values, which are the square root of the transmission eigenvalues. Then we use the left inverse of $t$, which is given by $(t^\dagger t)^{-1}t^\dagger = V_n(\Sigma_n^\dagger\Sigma_n)^{-1}\Sigma_n^\dagger U_n^\dagger$. Next we truncate the singular values by keeping only the first 500 diagonal elements in $(\Sigma_n^\dagger\Sigma_n)^{-1}\Sigma_n^\dagger$ (corresponding to keeping the reciprocal of 500 highest singular values), and replacing the remaining 524 diagonal elements of $(\Sigma_n^\dagger\Sigma_n)^{-1}\Sigma_n^\dagger$ by zero. Finally we build the angular memory operator $Q(\tilde{\theta}_i, \tilde{\theta}_o) = (t^\dagger t)^{-1}t^\dagger X^\dagger(\tilde{\theta}_o)tX(\tilde{\theta}_i)$ and find its eigenvectors. The

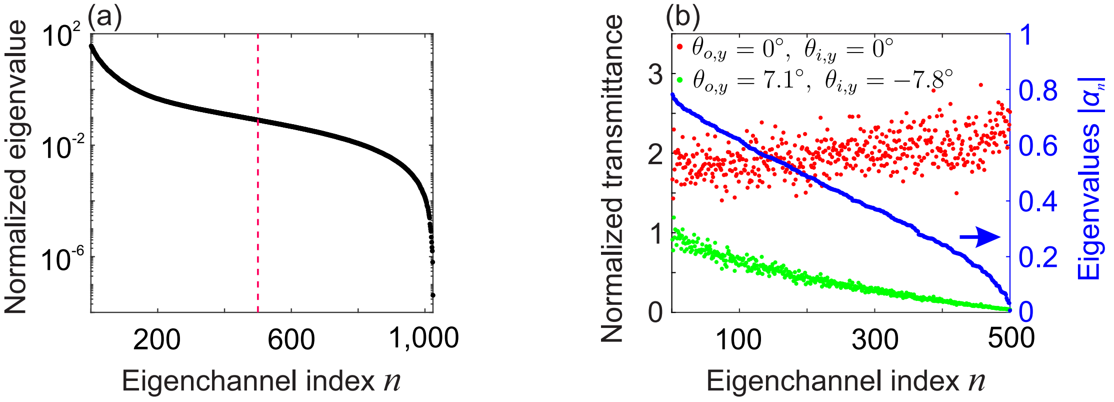


FIG. S5. **Transmission matrix truncation.** **(a)** The square of the singular values of the $N_o \times N_i = 1,024 \times 1,024$ transmission matrix $t$ in Fig. 3 of the main text represent the transmittance (transmission eigenvalues) of 1024 transmission eigenchannels. The red vertical line denotes the threshold we choose to discard 524 transmission eigenchannels with a transmittance below it. Phase-only-modulated angular memory eigenstates that comprise only of 500 transmission eigenchannels with transmittance above the threshold have improved angular correlation $|C_E|$, as shown in Fig. 3(e,f) of the main text. **(b)** Transmittance of all angular memory eigenstates $T_n$ with the original (red) or tilted wavefronts (green) are normalized by that of transmittance of a random input wavefront. A larger eigenvalue amplitude $|\alpha_n|$ (blue) corresponds to a higher transmittance for the tilted wavefronts, while the transmittance for the original (untilted) wavefront is nearly constant.

truncated matrix inversion results in using the 500 highest-transmission eigenchannels to construct the eigenvectors of $Q$, making them robust to phase-only modulation in our experiment.

Fig. S5(a) shows all transmission eigenvalues, corresponding to the transmittance of 1024 transmission eigenchannels. The red vertical line marks the threshold we choose for the truncated matrix inversion in Fig. 3(d-f) of the main text. 524 transmission eigenchannels with a transmittance below this threshold are discarded. The remaining 500 transmission eigenchannels constitute the eigenvectors of $Q$ operator. The angular correlation $|C_E|$ is significantly improved, as shown in Fig. 3(e) of the main text. The eigenstates with higher $|\alpha_n|$ have stronger correlation, because they have less contributions from lower transmission eigenchannels. This is confirmed by their transmittance shown in Fig. S5(b). The truncated matrix inversion is also used to obtain the results in Figs. 4 and S8 where we experimentally display the phase fronts of the eigenvectors on the SLM.

## I. Angular correlation measurement

After finding the eigenstates of $Q$, we display the phase pattern of the first eigenstate with the highest eigenvalue amplitude on the 1024 macropixels of the SLM, and measure the phase pattern of the light field transmitted through the sample with four-phase-shift interferometry method. We gradually shift the phase pattern of the eigenvector on the SLM to tilt its wavefront incident on the sample, and measure the transmitted phase patterns for each tilt angle of input $\theta_i$. Although the transmission matrix is measured with SLM macropixels (each containing $9 \times 9$ pixels), we laterally shift the input phasefront with the step size of *single* pixel on the SLM. Thus the input tilt angle is scanned at the step size of 0.29°. The scanning range is $(-10°, 10°)$, significantly larger than the angular correlation range $\delta\theta = 1.7°$ of the random wavefronts. Then we block the reference beam using a beam shutter, and measure the transmitted intensity pattern to recover the complex field profile. We repeat this measurement with a random incident wavefront to obtain the correlation function for conventional angular memory effect.

In the main text, we state two causes of the off-diagonal tilt of the measured angular correlation in Fig. 4: (i) refractive index mismatch on the input and output sides of the sample, and (ii) unequal sampling rate of input and output angles. Below we illustrate (ii) in a numerical simulation. Experimentally the sampling step of input tilt angle $\theta_i$ is larger than that of output tilt angle $\theta_o$ (given by the CCD camera pixel size). The measured angular correlation function $C_E$ can be simulated by convolution with the input and output angular point spread function (PSF). If the sampling step of $\theta_i$ is equal to that of $\theta_o$, the 2D PSF is isotropic and represented by a circle in Fig. S6(a). The convolved correlation is along the white line whose slope is equal to the ratio $n_i/n_o$ of refractive indices at input and output sides of the sample. However, when the input sampling step is larger than the output one, the 2D PSF is elongated horizontally, and the convolved correlation is tilted slightly towards the horizontal axis. This result agrees with the experimental data in Fig. 4 in the main text, confirming the effect of sampling rate on the angular correlation

function.

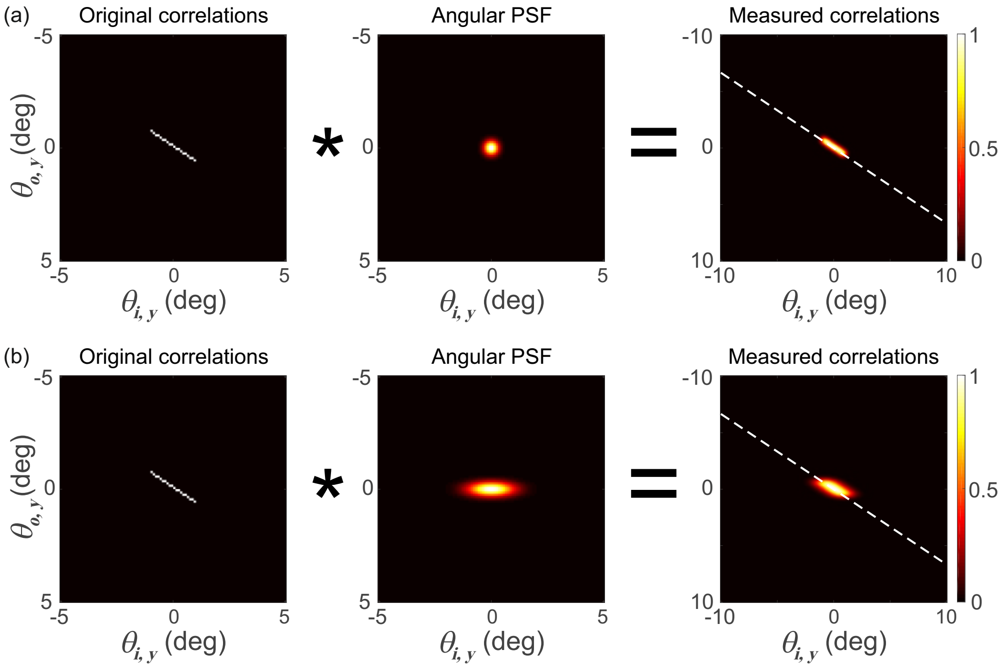


FIG. S6. **Effect of sampling rate on the angular correlation function.** The first column shows the angular correlation function tilted away from the diagonal due to refractive index mismatch at input and output sides of the sample. The second column shows the angular PSF, which is determined by the sampling steps of input and output angles. The last column is simulation of measured correlation function which is a convolution of the first and second columns. **(a)** The sampling steps of input and output angles are identical, the angular PSF is isotropic, and the tilt of the angular correlation function from the diagonal is determined by the refractive index mismatch (dashed white line). **(b)** The sampling step of input angle is larger than that of output angle, the PSF is elongated horizontally, and the correlation function is tilted further towards the horizontal axis.

### J. Creating double memories

In the main text, we create the angular memory simultaneously at two pairs of input and output tilt angles, by setting the incident wavefront to an eigenstate of a joint operator $Q_{1+2} = [Q_1(\tilde{\theta}_{i,1}, \tilde{\theta}_{o,1}) + Q_2(\tilde{\theta}_{i,2}, \tilde{\theta}_{o,2})]/\sqrt{2}$. Alternatively, double memories can be obtained by superposing the eigenstates of the two operators $(V_n^{(1)} + V_n^{(2)})/\sqrt{2}$, where $Q_1 V_n^{(1)} = \alpha_n^{(1)} V_n^{(1)}$ and $Q_2 V_n^{(2)} = \alpha_n^{(2)} V_n^{(2)}$.

We compute the angular correlations in these two cases, and compare to that of single memory. Fig. S7(a) shows the correlation coefficient $|C_E(\theta_{i,y}, \theta_{o,y})|$ for the first eigenvector $V_1^{(1)}$ of $Q_1(\tilde{\theta}_{i,y} = 7.8°, \tilde{\theta}_{o,y} = -3.5°)$ with the largest eigenvalue amplitude $|\alpha_1^{(1)}|$. The maximum correlation at $\theta_{i,y} = \tilde{\theta}_{i,y} = 7.8°, \theta_{o,y} = \tilde{\theta}_{o,y} = -3.5°)$ is $|C_E| = 0.88$. In Fig. S7(b), we compute the angular correlation for the incident wavefront $(V_1^{(1)} + V_1^{(2)})/\sqrt{2}$, where $V_1^{(2)}$ is the first eigenvector of $Q_2(\tilde{\theta}_{i,y} = -7.8°, \tilde{\theta}_{o,y} = 7.1°)$ with the largest eigenvalue amplitude $|\alpha_1^{(2)}|$. The maximum correlations at the preselected angles, $|C_E(7.8°, -3.5°)| = |C_E(-7.8°, 7.1°)| = 0.46$, are reduced approximately by a factor of 2 from that of single memory in Fig. S7(a). Fig. S7(c) shows the angular correlation for the incident wavefront being the first eigenvector of the joint operator $Q_{1+2}$ which has the largest eigenvalue amplitude $|\alpha_1^{(1+2)}|$. The correlations at the two pairs of designated angles are $|C_E(7.8°, -3.5°)| = 0.68$ and $|C_E(-7.8°, 7.1°)| = 0.63$. Hence, the decrease from the single memory is about $\sqrt{2}$. These results confirm that it is more efficient to create double memories with the eigenvectors of the joint angular memory operator than superposing the eigenvectors of separate operators.

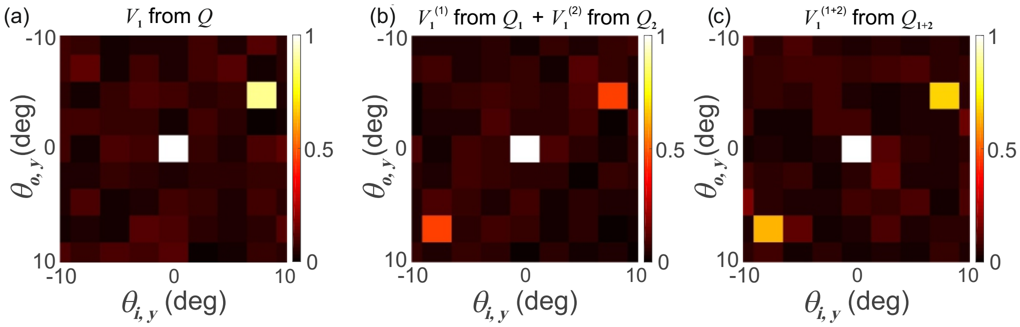


FIG. S7. **Single memory versus double memories.** **(a)** Angular correlation $|C_E(\theta_{i,y}, \theta_{o,y})|$ for the incident wavefront equal to the first eigenvector $V_1^{(1)}$ of the angular memory operator $Q_1(\tilde{\theta}_{i,y} = 7.8°, \tilde{\theta}_{o,y} = -3.5°)$. The number of controlled input channels is $N_i$ = 1,024, and the number of detected output channels is $N_o$ = 4,096. **(b)** Superposing the first eigenvectors of two operators $Q_1(\tilde{\theta}_{i,y} = 7.8°, \tilde{\theta}_{o,y} = -3.5°)$ and $Q_2(\tilde{\theta}_{i,y} = -7.8°, \tilde{\theta}_{o,y} = 7.1°)$ in the incident wavefront reduces the maximum correlation by a factor of 2 to $|C_E| = 0.46$. **(c)** The first eigenvector of a joint operator $Q_{1+2} = (Q_1 + Q_2)/\sqrt{2}$ enhances the correlations at two pairs of input and output angles: $|C_E(7.8°, -3.5°)| = 0.68$ and $|C_E(-7.8°, 7.1°)| = 0.63$. These values are roughly a factor of $\sqrt{2}$ lower than that of single memory in (a).

## K. Two special cases

Finally, we investigate the eigenstates of the angular memory operator in two special cases: (i) output tilt angle $\tilde{\theta}_o = 0$; (ii) input tilt angle $\tilde{\theta}_o = 0$.

For comparison, we show the experimentally measured $|C_E(\theta_i, \theta_o)|$ for a random phase front of the input field in Figs. S8(a-c). In (a), $|C_E|$ exhibits conventional memory effect correlation around the origin ($\theta_i = 0, \theta_o = 0$). The autocorrelation functions of input field pattern in (b) and of output in (c) vanish away from the origin, indicating there is no spatial correlation in the input or the output wavefront.

Fig. S8(d), which is the same as Fig. 4(a) of the main text, shows the measured $|C_E(\theta_i, \theta_o)|$ for the first eigenstate of angular correlation operator $Q(\tilde{\theta}_{i,y} = -7.8°, \tilde{\theta}_{o,y} = 7.1°)$. The autocorrelation functions of the input and output field profiles in (e) and (f) are identical to those of a random input. Hence, there is no correlation in both the input and the output field patterns for this eigenstate with $\tilde{\theta}_i \neq 0$ and $\tilde{\theta}_o \neq 0$.

Fig. S8(g-i) represent the first special case: $\tilde{\theta}_{i,y} = -7.8°$, $\tilde{\theta}_{o,y} = 0$. In Fig. S8(g), the experimentally measured $|C_E|$ is enhanced not only at $(\theta_{i,y} = -7.8°, \theta_{o,y} = 0)$ as intended, but also at $(\theta_{i,y} = 7.8°, \theta_{o,y} = 0)$. This phenomenon originates from the periodic modulation of the input field, as confirmed by the autocorrelation function of the input field pattern in (h), which reveals the modulation period is equal to 7.8°. The output field pattern has no spatial correlation, as seen from its autocorrelation function in (i).

Fig. S8(j-l) illustrate the second special case: $\tilde{\theta}_{i,y} = 0$, $\tilde{\theta}_{o,y} = -7.1°$. $|C_E|$ is enhanced not only at $(\theta_{i,y} = 0, \theta_{i,y} = -7.1°)$ as intended, but also at $(\theta_{i,y} = 0, \theta_{i,y} = 7.1°)$ in Fig. S8(j). According to its autocorrelation function in Fig. S8(l), the output field pattern is periodically modulated with a period of 7.1°. The input field pattern has no correlation, as confirmed by its autocorrelation function in Fig. S8(k).

These two special cases are examples of encoding angular memories into the input or output wavefronts.

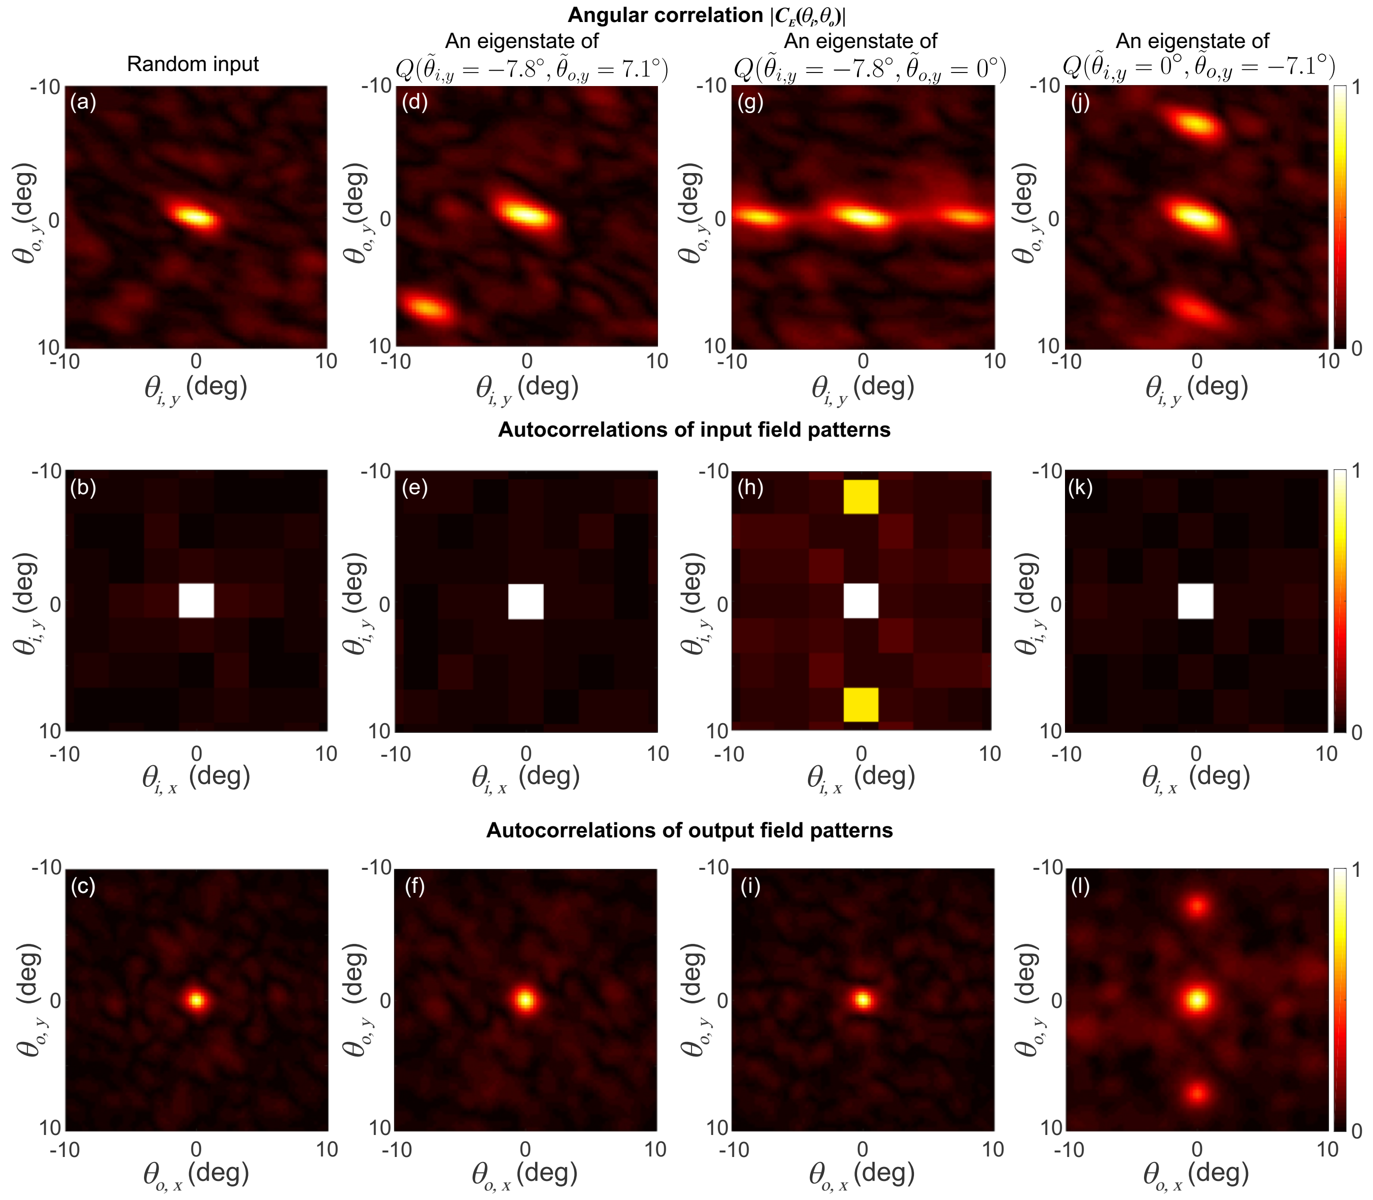


FIG. S8. **The angular memories and the autocorrelations of the input and the output fields.** First row: correlation coefficient $|C_E(\theta_{i,y},\theta_{o,y})|$ is shown, where $\theta_{i,y}$ represents the input tilt angle, and $\theta_{o,y}$ the output tilt angle in $y$ direction. The input wavefront is random in **(a)**, equal to an angular memory eigenstate of $Q(\tilde{\theta}_{i,y}=-7.8°,\tilde{\theta}_{o,y}=7.1°)$ in **(d)**, $Q(\tilde{\theta}_{i,y}=-7.8°,\tilde{\theta}_{o,y}=0)$ in **(g)**, $Q(\tilde{\theta}_{i,y}=0,\tilde{\theta}_{o,y}=-7.1°)$ in **(j)**. Second row: autocorrelations of input field patterns for (a,d,g,j) are shown in **(b,e,h,k)**, revealing periodic modulation of input field in (h). Third row: autocorrelations of output field patterns for (a,d,g,j) are shown in **(c,f,i,l)**, revealing periodic modulation of output fields in (l). The rest input and output field patterns have no spatial correlations. $N_i=1024$, $N_o=4096$. Here, we use the truncated matrix inversion by keeping the first 500 singular vectors with the highest 500 singular values. In all cases, we experimentally display the phase front of the eigenvector with the highest eigenvalue $|\alpha_n|$ and measure the output field patterns with the four-phase-shift interferometry method.
